# Supplementary material for: Quantum measurement of a rapidly rotating spin qubit in diamond
Source: arXiv:1802.03512 source file (2018-02-10)
Supplement: Supplementary file 1 [file Movingnvs_supp.pdf]

# Quantum measurement of a rapidly rotating spin qubit in diamond-SUPPLEMENTARY INFORMATION

Alexander A. Wood,[1] Emmanuel Lilette,[1] Yaakov Y. Fein,[1] Nikolas Tomek,[2] Liam P. McGuinness,[2] Lloyd C. L. Hollenberg,[1] Robert E. Scholten,[1] and Andy M. Martin[1,*]

[1]*School of Physics, University of Melbourne, Victoria 3010, Australia*

[2]*Institut für Quantenoptik, Universität Ulm, Ulm 89069, Germany*

(Dated: December 15, 2017)

* martinam@unimelb.edu.au

## S1. STATIONARY SPIN-ECHO SIGNAL

At the magnetic bias field strengths considered in this work, the residual $^{13}$C nuclear spins in the diamond (about 0.2 %) modulate the spin echo signal at half the $^{13}$C precession frequency (3.33 kHz). We determine the field-dependent [1, 2] spin coherence time $T_2$ from the data as the time constant to the overall envelope of the collapse-revival spin-echo signal from stationary measurements. Supplementary Figure 1 shows the spin-echo signal at a magnetic field strength of 6.2 G, taken from NV1 when stationary.

The fitted decay time from the data of Supplementary Figure 1 and repeated experiments is determined to be $T_2 = 352\,\mu s$. Spin-echo interrogation times for experiments described in the main text are limited to times within the initial collapse of the echo signal (which is entirely suppressed for $\tau > 100\,\mu s$). In rotating experiments, we did not observe any spin-echo revival. The primary factor responsible is the effective AC magnetic field due to a mutual misalignment of the bias magnetic field and NV axis (fixed at 54.7°) from the rotation axis (Eq. 1 of the main text). For a $\tau = 300\,\mu s$ spin-echo interrogation time, $B_0 = 6.2$ G and the diamond rotating at 3.33 kHz, the spin-echo phase accumulated is $\pi$ for only a 0.01° magnetic field misalignment from the rotation axis. With our apparatus it was not possible to control the alignment to such precision, leading to an effective AC magnetic field with random amplitude and phase that suppressed the revival when rotating. Another factor in the non-observation of the echo revival when rotating is due to rotationally-induced shifts of the nuclear spin precession frequency [3] which were not characterised when the experiments

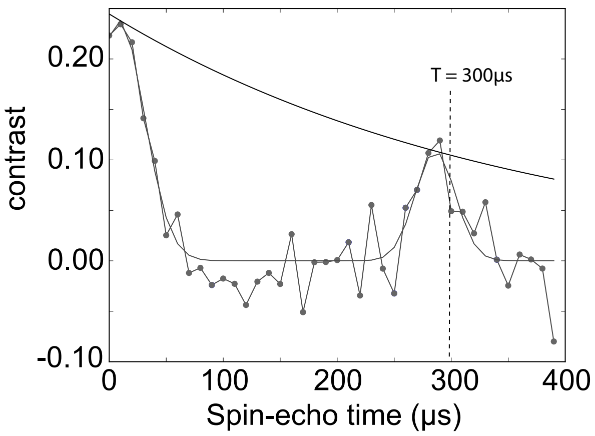


Supplementary Figure 1. Spin-echo signal from NV1 at B = 6.2 G, showing revival near 300 µs and $^{13}$C dominated $T_2$ damping, with characteristic timescale $T_2 = 352\,\mu s$.

in this work were conducted.

## S2. EFFECT OF PULSE DURATION

The NV centre used in our experiments, NV1, is located about 10μm from the centre of rotation. It therefore exhibits circular motion, and has a significant tangential velocity ($25\,\mathrm{cm\,s^{-1}}$ at 3.33 kHz). The duration of the laser pulse in our strobed confocal microscopy experiments determines the angular displacement of the NVs during imaging. The minimum laser pulse time we use is 2 μs. For shorter pulse durations the signal to noise of the resulting images is substantially lower than that presented in the main text. Longer pulse durations lead to 'smearing' of the emitted fluorescence during a strobed confocal image, as shown in Supplementary Figure 2.

Random jitter of the motor period broadens the fluorescence along the rotation arc shown in Supplementary Figure 2. From stationary confocal images, we fit a Gaussian model to determine the characterisitic width of the spatial profile, and find $(\sigma_x, \sigma_y) = (286, 291)\,\mathrm{nm}$, with $\sigma_i$ the $1/e^2$ radius. Analysing time-dependent photoluminesence traces of the NV moving under the laser beam reveals a characteristic temporal width of $\sigma_{\mathrm{pl,t}} = 2.6\,\mu\mathrm{s}$. Using the tangential speed of the NV, the average spatial width $\tilde{\sigma} = 289\,\mathrm{nm}$ can be converted to an equivalent temporal width, $\tilde{\sigma}_{\mathrm{t}} = 1.3\,\mu\mathrm{s}$. We simulate period jitter of the motor by sampling random shifts of the mean value (center) of the temporal intensity profile with intrinsic

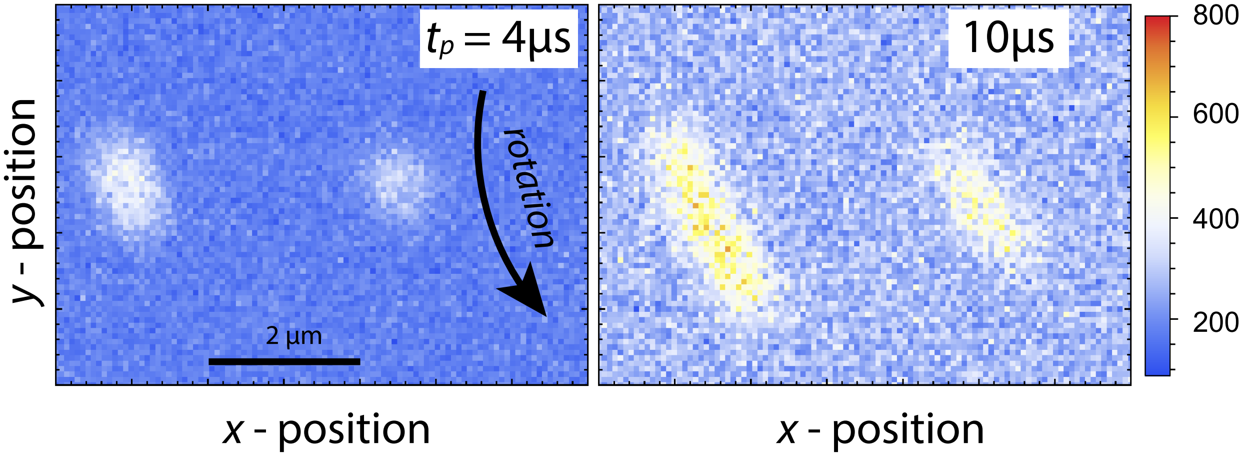


Supplementary Figure 2. Longer pulse durations smear the emitted fluorescence. Left: a 4 μs laser pulse and, right, a 10 μs laser pulse.

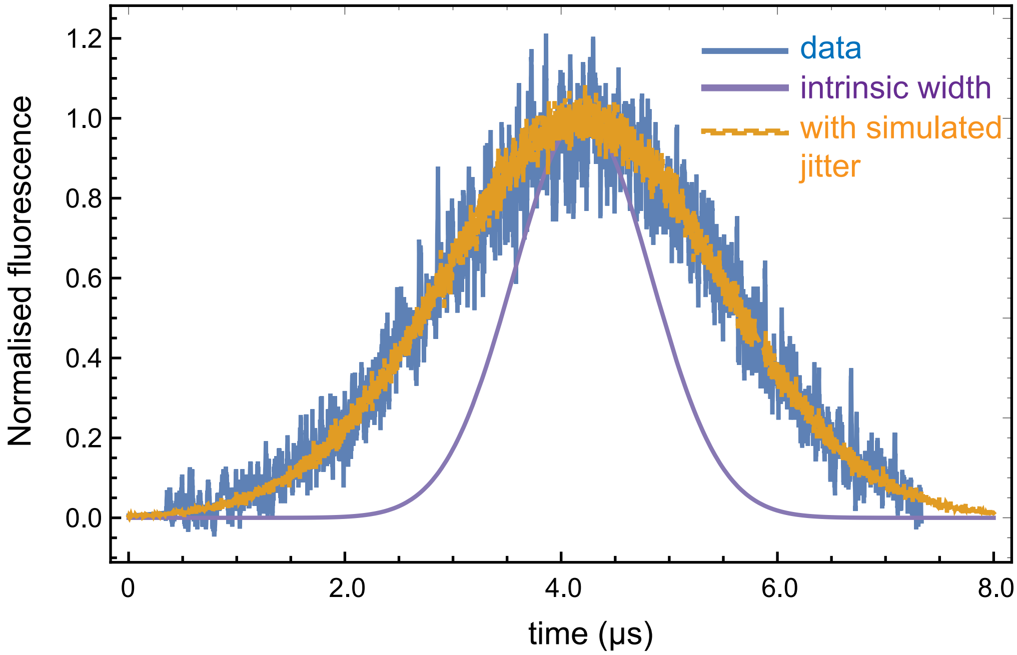


Supplementary Figure 3. Estimation of motor period jitter. Fluoresence is collected from an NV moving under the laser beam (blue data points). We then determine from fits to stationary confocal images of a single NV centre the equivalent temporal width $\tilde{\sigma}_\mathrm{t}$ the NV would be expected to exhibit as it moved under the laser, assuming no jitter (purple). We then simulate jitter of the motor period by averaging the result of many simulated fluoresence traces with the same intrinsic width $\tilde{\sigma}_\mathrm{t}$ but variable mean position. The random shifts are drawn from a normal distribution centred at 0 with a width given by $\sigma_\mathrm{jitter}$.The value of $\sigma_\mathrm{jitter}$ is determined by fitting the simulation to the data, giving $\sigma_\mathrm{jitter} = 1.1\,\mu\mathrm{s}$.

width $\tilde{\sigma}_\mathrm{t}$ from a normal distribution of width $\sigma_\mathrm{jitter}$ and adjust $\sigma_\mathrm{jitter}$ until the width of the fluoresence over many averages corresponds to that measured in rotating photoluminesence experiments (Supplementary Figure 3). We find that the motor period exhibits a standard deviation of 1.1 μs over a 15 min averaging period, corresponding to a 0.4% error in the motor period. For individual consecutive periods of the motor we typically observe period variations on the order of a few hundred nanoseconds.

While period jitter of the motor broadens the strobed confocal images (and photoluminesence time traces), wobble of the axis broadens the confocal images radially. For pulse durations of 2 μs, it can be observed that the radial broadening and azimuthal smearing are approximately equal, suggesting horizontal wobble on the order of a few hundred nanome-

tres.

## S3. TIME-DEPENDENT OPTICAL PUMPING OF THE NV

During optical preparation and readout the NV sees a time-dependent intensity due to the approximately Gaussian spatial profile of the laser beam. The state-dependent fluorescence that makes the NV so useful as a quantum bit is sensitive to the time dependence of the laser intensity.

We simulated the state-dependent photoluminescent response to time-dependent optical pumping using the theoretical models outlined in Refs. [4, 5]. In the absence of a magnetic field, the NV is modelled as a seven-level system: the single bright and two dark states in the ground state manifold ($|0\rangle$, $|1\rangle$ and $|2\rangle$), the complementary states in the excited state manifold ($|3\rangle$, $|4\rangle$ and $|5\rangle$) and the singlet state in the non-radiative transition pathway ($|6\rangle$). The rate equations for the state populations $n_i$ are given by

$$\frac{\partial n_i}{\partial t} = \sum_{j=0}^{6} (k_{ij} n_j - k_{ij} n_i) \tag{1}$$

with the relaxation rates and pumping rates connecting different states $i$ and $j$ denoted by $k_{ij}$. We determined that $k_{30} = k_{41} = k_{52} = 6.5 \times 10^7\,\mathrm{s}^{-1}$, $k_{36} = 1.1 \times 10^7\,\mathrm{s}^{-1}$, $k_{46} = k_{56} = 3 \times 10^7\,\mathrm{s}^{-1}$, $k_{60} = 3 \times 10^6\,\mathrm{s}^{-1}$ and $k_{61} = k_{62} = 1.3 \times 10^6\,\mathrm{s}^{-1}$ for the relaxation rates and $k_{03} = \beta(t)k_{30}$, $k_{14} = \beta(t)k_{41}$ and $k_{25} = \beta(t)k_{52}$ for the pumping rates best described the photoluminesence traces observed in our experiments. Here, $\beta(t)$ is a truncated Gaussian function with $1/e$ width $\approx 1\,\mu\mathrm{s}$, which matched the measured data reasonably well.

A particularly important degree of freedom in our experiment is the time at which the laser illumination is switched on: although the NV is constantly moving, we can adjust the trigger delay time $t_D$ that controls when the NV enters the laser preparation region. The NV can then either move gradually through the beam, in which case the emitted fluorescence would appear to be Gaussian, or we could turn the laser beam on as the NV is immediately below the highest intensity point, and the emitted fluorescence is approximately a truncated Gaussian. The state-dependent pumping dynamics that give rise to state contrast, and therefore the ability to determine the NV state, depend on this delay time $t_D$. Supplementary Figure 4 shows the simulated state contrast (bright state-dark state fluorescence) as a function of the measurement and delay times as well as the corresponding time traces at

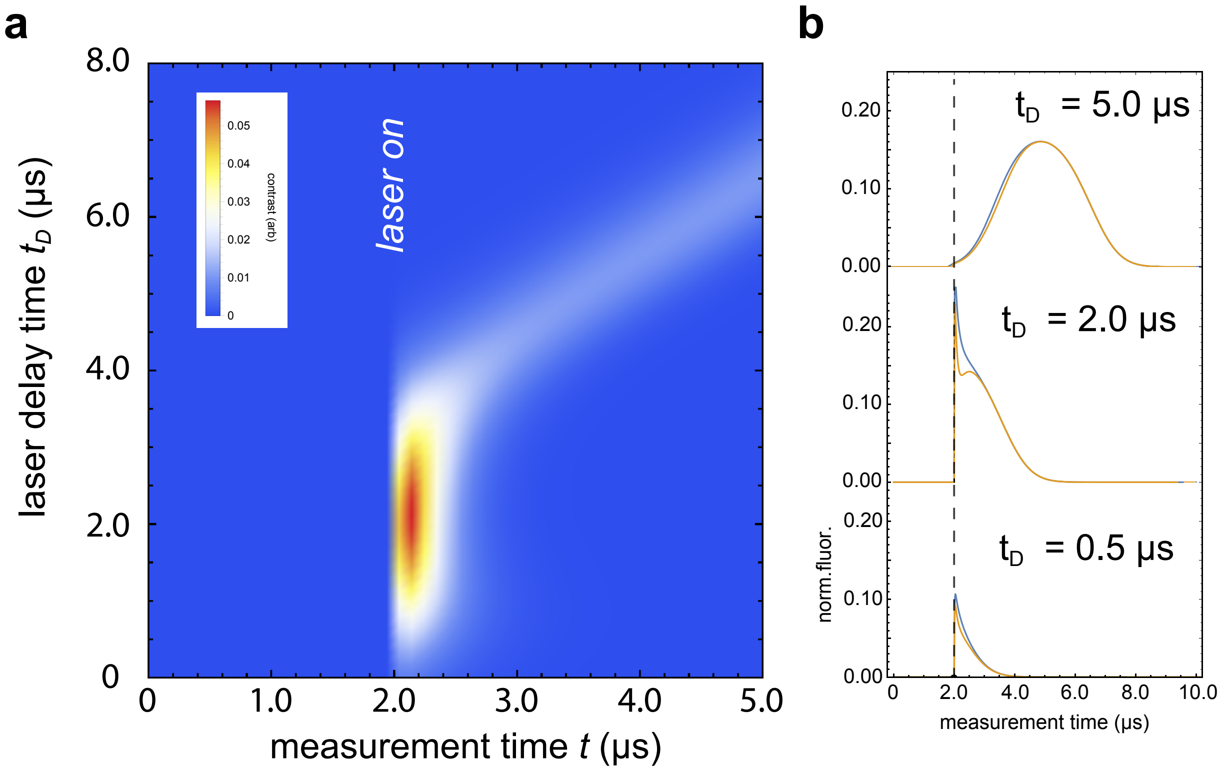


Supplementary Figure 4. Dependence of NV contrast on delay time. (a) State contrast (bright state minus dark state fluorescence) as a function of measurement time $t$ and delay time $t_D$. In this simulation, the laser is turned on at $t = 2.0\,\mu$s. (b) Simulated fluorescence time traces for the bright and dark NV states as a function of measurement time $t$ for delay times of $t_D = 0.5$, 2.0 and 5.0 µs. Curves are displaced vertically for clarity. The state contrast is optimised for $t_D = 2\mu$s, corresponding to the NV being directly below the laser illumination region when it is switched on and thus seeing the peak spatiotemporal intensity.

three delay times. It is clearly evident that unless the laser illumination is switched on (in this case, always at $t = 2.0\,\mu$s) when the NV is directly below it, the fluorescence contrast is significantly reduced.

## S4. DRIFT DURING EXPERIMENTS

Due to the small number of photons collected during each laser pulse, experiments must be repeated many ($> 10^5$) times to obtain statistically significant results. The sensitivity of the fluorescence contrast to the position of the NV demands minimal spatial drift during

experimental averaging time. Slow ($< 1\,$hr) ambient temperature drifts driving thermal expansion of the motor axle and its associated internal mounting result in the position of the NV varying during and between measurements. Since the timing of pulses was unchanged during this drifting, the NV position drift corresponds to an effective variation in the delay time $t_D$ away from the optimum value for maximum state contrast ($t_D = 2\,\mu$s in Supplementary Figure 4). Thus, not only does drift result in a reduction of signal photons collected, it additionally leads to variation of the maximum state contrast, a far more significant problem. To minimise the signal loss, the laser was periodically refocused on the NV centre between experiments. After a few hours of warm-up time, the motor internal temperature stabilises to around 60°C (with the diamond about 10° cooler) and the position of the NV was observed to drift by 0.5 µm/hr in the $x - y$ plane and 0.7 µm/hr in $z$. We were able to interrogate the NV for up to 10 min before refocusing the objective on the new NV position.

## REFERENCES


[1] N. Zhao, S.-W. Ho, and R.-B. Liu, Decoherence and dynamical decoupling control of nitrogen vacancy center electron spins in nuclear spin baths. Phys. Rev. B **85**, 115303 (2012).

[2] L. T. Hall, J. H. Cole, and L. C. L. Hollenberg, Analytic solutions to the central-spin problem for nitrogen-vacancy centers in diamond. Phys. Rev. B **90**, 075201 (2014).

[3] A. A. Wood, E. Lilette, Y. Y. Fein, V. S. Perunicic, L. C. L. Hollenberg, R. E. Scholten, and A. M. Martin, Magnetic pseudo-fields in a rotating electron-nuclear spin system. Nature Physics **13**, nphys4221 (2017).

[4] N. B. Manson, J. P. Harrison, and M. J. Sellars, Nitrogen-vacancy center in diamond: Model of the electronic structure and associated dynamics. Phys. Rev. B **74**, 104303 (2006).

[5] J.-P. Tetienne, L. Rondin, P. Spinicelli, M. Chipaux, T. Debuisschert, J.-F. Roch, and V. Jacques, Magnetic-field-dependent photodynamics of single NV defects in diamond: an application to qualitative all-optical magnetic imaging. New J. Phys. **14**, 103033 (2012).
